# Supplementary material for: Channel-Attentive Graph Neural Networks
Source: arXiv:2503.00578 source file (2025-03-05)
Supplement: Supplementary file 1 [file appendix.tex]

\appendix

\section{Channel Weights at Deeper Layers}
\label{apx:channel_weight}

We present visualizations of pairwise cosine similarities of channel weights for five randomly selected nodes. We limit the number of nodes because of space limitations. We have observed similar results for all nodes. The visualizations for four datasets can be seen in Figures~\ref{fig:heatmap_more_1},~\ref{fig:heatmap_more_2},~\ref{fig:heatmap_more_3}. The results are obtained from all layers of the best models, which we report the results of in Table~\ref{tab:benchmark}. 

For highly heterophilous datasets, we can observe that nodes send different messages to their neighbors. Figures~\ref{fig:heatmap_more_1} and ~\ref{fig:heatmap_more_2} show that, in Minesweeper and Roman-Empire datasets, the message-passing scheme changes with respect to different nodes and layers. This shows that CHAT-GNN leverages the channel-attentive mechanism to differentiate the sent messages between neighbors.

We also observe that nodes send almost identical messages to their neighbors in graphs with high homophily. In Figure~\ref{fig:heatmap_more_3}, we show that the nodes send identical messages to their neighbors in Pubmed. The messages become different in some cases for the second layer.
% \begin{figure*}[t]
%   \parbox{\linewidth}{
%     \centering
%     \includegraphics[width=0.9\linewidth]{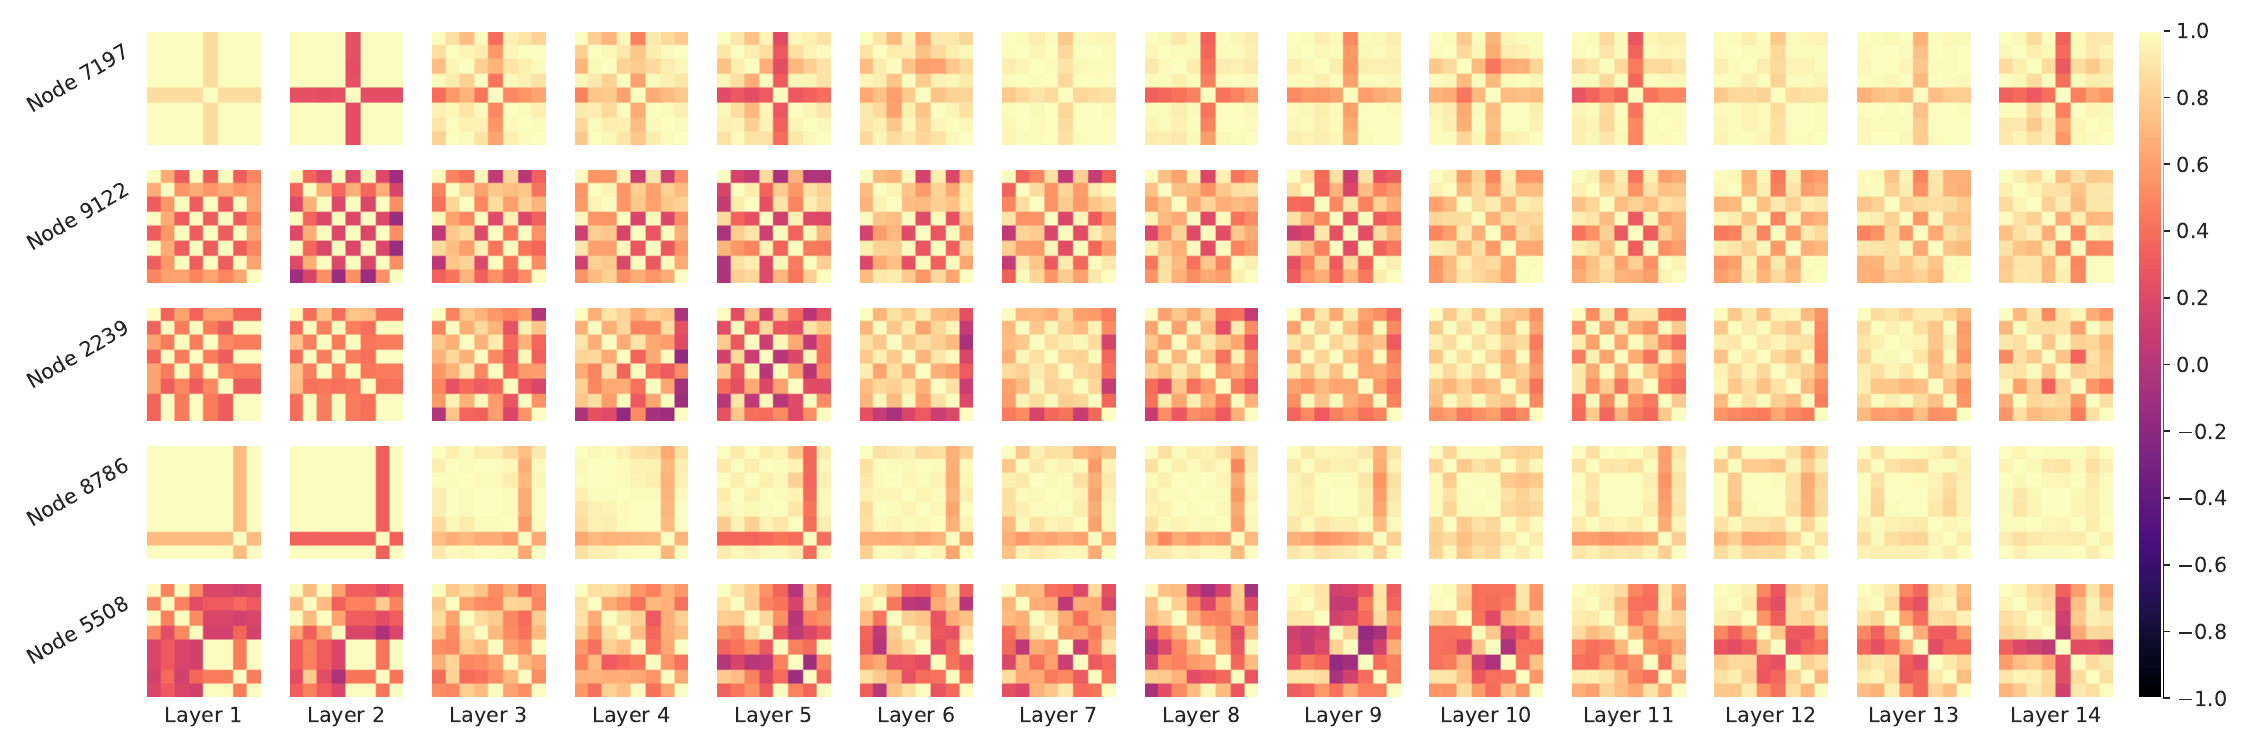}
%   }
%   \caption{Visualization of pairwise cosine similarities of channel attention vectors at deeper layers for Minesweeper dataset.}
%   \label{fig:heatmap_more_1}
% \end{figure*}
% \begin{figure*}[t!]
%   \parbox{\linewidth}{
%     \centering
%     \includegraphics[width=0.9\linewidth]{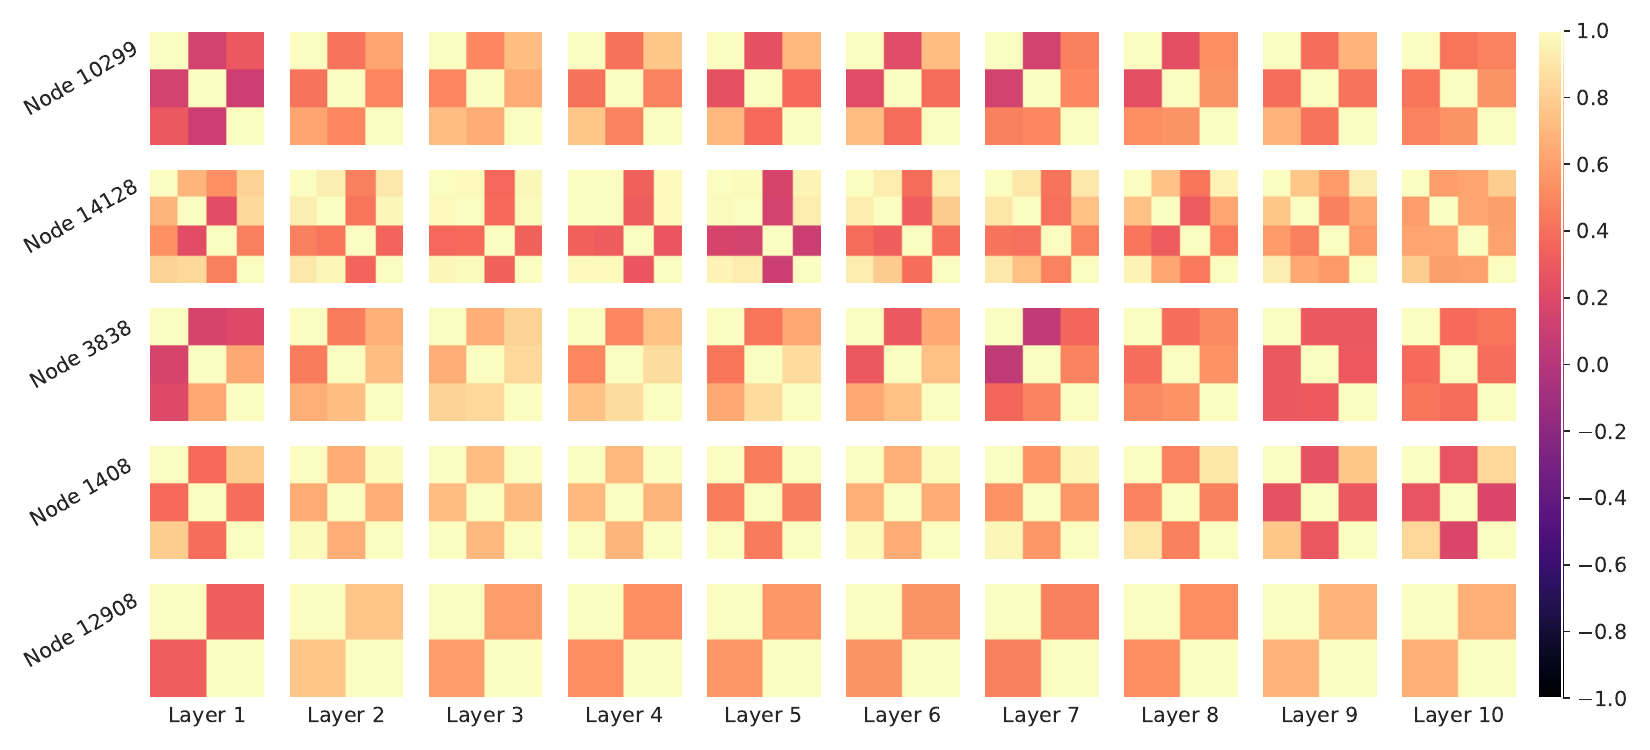}
%   }
%   \caption{Visualization of pairwise cosine similarities of channel attention vectors at deeper layers for Roman-Empire dataset.}
%   \label{fig:heatmap_more_2}
% \end{figure*}

\begin{figure*}[t]
    \centering
    \includegraphics[width=\linewidth]{images/chatgnn_minesweeper_att_vecs_heatmap.pdf}
  \caption{Visualization of pairwise cosine similarities of channel attention vectors at deeper layers for Minesweeper dataset.}
  \label{fig:heatmap_more_1}
\end{figure*}
\begin{figure*}[t]
    \centering
    \includegraphics[width=\linewidth]{images/chatgnn_roman-empire_att_vecs_heatmap.pdf}
  \caption{Visualization of pairwise cosine similarities of channel attention vectors at deeper layers for Roman-Empire dataset.}
  \label{fig:heatmap_more_2}
\end{figure*}

\begin{figure*}[t]
  \parbox{0.49\linewidth}{
    \centering
    \includegraphics[width=\linewidth]{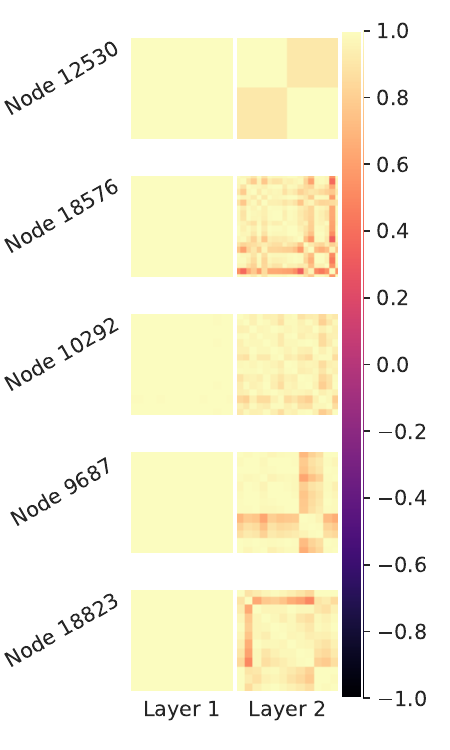}
  }
  \parbox{0.49\linewidth}{
    \centering
    \includegraphics[width=\linewidth]{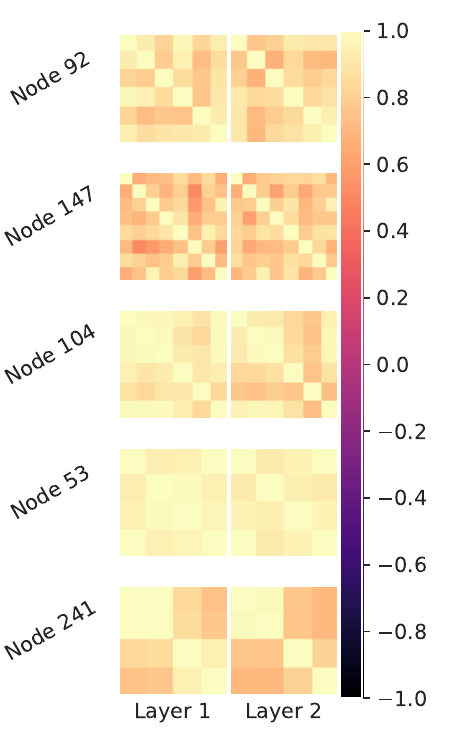}
  }
  \caption{Visualization of pairwise cosine similarities of channel attention vectors at deeper layers for Pubmed and Wisconsin datasets.}
  \label{fig:heatmap_more_3}
\end{figure*}
